# Supplementary material for: Nonreciprocal Coulomb Drag between Quantum Wires in the quasi-1D regime
Source: arXiv:2310.13626 ancillary file (2024-01-17)
Supplement: Supplementary file 1 [file Supplement_CD_resubmission.pdf]

# Supplemental Material for "Non-reciprocal Coulomb Drag between Quantum Wires in the quasi-1D regime"

Rebika Makaju,[1] Hafsa Kassar,[1] Sabahattin M. Daloglu,[1] Anna Huynh,[1]
Alex Levchenko,[2] Sadhvikas J. Addamane,[3] and Dominique Laroche[1,*]

[1] *Department of Physics, University of Florida, Gainesville, FL 32611, USA*
[2] *Department of Physics, University of Wisconsin–Madison, Madison, WI 53706, USA.*
[3] *Center for Integrated Nanotechnologies, Sandia National Laboratories, Albuquerque, NM 87185, USA*

## I. DEVICE FABRICATION

A n-doped AlGaAs/GaAs heterostructure (VA182) with the 2DEG burried 80 nm below the surface is used as a starting point to fabricate the laterally coupled quantum wires. A mesa structure is patterned using standard photolithography techniques and defined using a wet phosphoric acid etch. Ohmic contacts (Ge/Au/Ni/Au of thickness 260 Å/ 540 Å/ 140 Å/ 960 Å-) are then defined using photolithography and sputtered into the heterostructure, followed by an annealing step at $420°C$ for 1 min in a rapid thermal annealer. Finally e-beam lithography is utilized to define the electrostatic gates (Ti-Au of thickness 100 Å- 1000 Å), which are deposited using sputtering. The quantum wires in the device are separated by 150 nm. A Scanning electron microscope image of a typical device is shown in Fig. 1(c) of the main text, and a schematic of the mesa with the gates and the ohmic contacts is presented in Fig. S1. The device is defined by three gates, $V_T$, $V_M$ and $V_B$, allowing for independent contacts to each quantum wire.

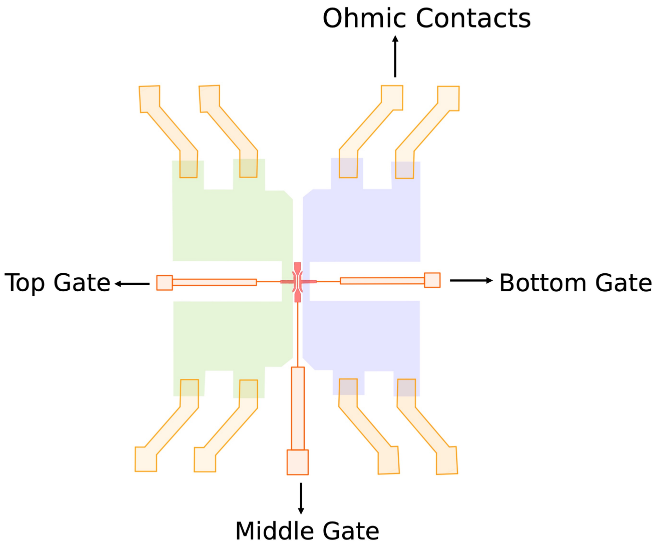


FIG. S1: Schematic of the mesa structure with the gates and the ohmic contacts.

## II. DEVICE CHARACTERIZATION

Before conducting Coulomb drag (CD) measurements, it is imperative to perform consistency tests to characterize the prospective drag signal. We carried out four different tests: *i)* Tunneling test, *ii)* Frequency independence, *iii)* Current linearity, and *iv)* Onsager reciprocity.

As a starting point for the consistency tests, the middle gate was swept with bias voltage. As seen from Fig. S2, the middle gate pinches off at $V_M < 0.2V$. The tunneling measurements, as shown in Fig. S3. $V_M$, were performed

---

* dlaroc10@ufl.edu

by sending a small source-drain voltage across the device for different $V_M$ values. $V_M$ was selected such that the tunneling resistance between the two wires was larger than $30M\Omega$.

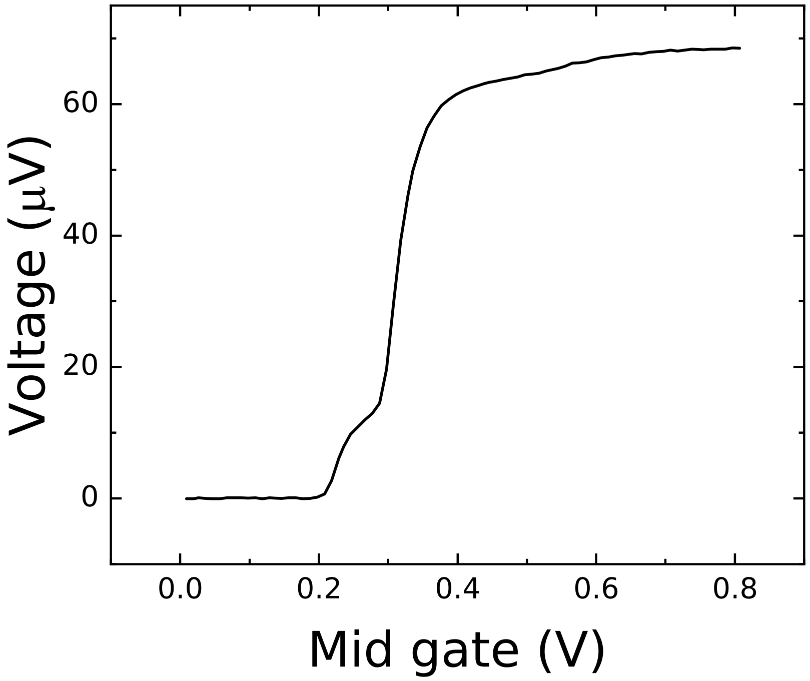


FIG. S2: Interwire voltage drop as a function of middle gate voltage.

The CD signal is expected to be independent of the frequency used, which is what we observed, as shown in Fig. S4. Frequencies ranging from 9 Hz to 85 Hz were tested. The other two standard tests for momentum-transfer induced Coulomb drag, current linearity and Onsager relations, are discussed in the main text, as they provide strong evidence for the presence of a rectified Coulomb drag signal between the quantum wires.

## III. SYMMETRIC AND ANTI-SYMMETRIC DRAG COMPONENTS

As discussed in the main text, the drag signal in our device does not follow Onsager relation, both upon layer reversal and upon current direction reversal. Fig. S5 shows the symmetric and anti-symmetric drag components with the bottom wire as drive wire and the top wire as the drag wire (Fig. 3 (c) and (d) in main text). While the anti-symmetric is non-zero, the signal appears to be dominated by the symmetric component, pointing towards the predominance of a rectified CD signal.

## IV. ONSAGER RELATION AT HIGH TEMPERATURE

As mentioned in the main text, Onsager's reciprocity was broken for both AC and DC drag. Figs. 3 and 5 were taken at the base temperature of the dilution refrigerator, with an electron temperature estimated to be 150 mK. We also tested the Onsager relation at higher temperatures, for both AC and DC drag, and the results remained similar. Thus, the Onsager's relation was broken at high temperatures for AC and DC drag, which are shown in Fig. S6 to Fig. S9.

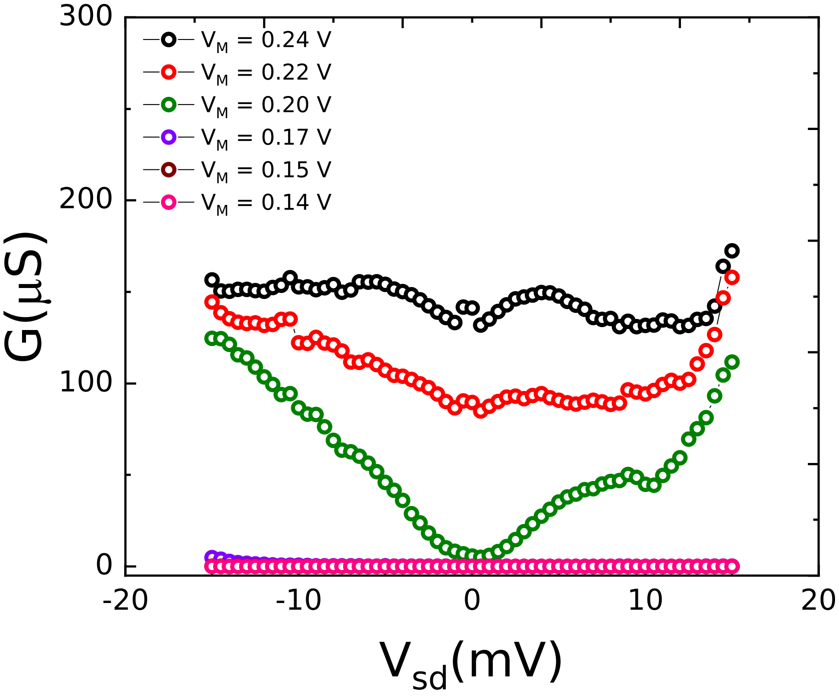


FIG. S3: Example of tunneling measurement with different middle gate voltages.

## V. DC CURRENT DEPENDENCE

In addition to the I-V curves shown in the main text, we plotted the drive current as a function of the DC drag voltages at different top gate voltages, as shown in Fig. S10. The I-V relation remained non-linear at different top gate voltages. The polynomial coefficients remained comparable for all top gate voltages, which are shown in Tables S1 and S2.

| $V_T(V)$ | B $(\mu V/nA)$ | C $(\mu V/nA^2)$ | D $(\mu V/nA^3)$ |
|---|---|---|---|
| -0.284 | -4.36755 | -0.00556 | $4.46112 \times 10^{-4}$ |
| -0.197 | -4.46002 | -0.00526 | $4.8994 \times 10^{-4}$ |
| -0.235 | -4.43805 | -0.00528 | $4.86312 \times 10^{-4}$ |
| -0.323 | -4.43393 | -0.00542 | $4.81029 \times 10^{-4}$ |

TABLE S1: Parameters obtained from fitting a cubic polynomial $y = Bx + Cx^2 + Dx^3$ for the wire setup as shown in Figure S10(a).

| $V_T(V)$ | B $(\mu V/nA)$ | C $(\mu V/nA^2)$ | D $(\mu V/nA^3)$ |
|---|---|---|---|
| -0.284 | -4.8619 | $-7.46574 \times 10^{-4}$ | $5.92456 \times 10^{-4}$ |
| -0.197 | -4.87953 | $-5.68605 \times 10^{-4}$ | $5.86824 \times 10^{-4}$ |
| -0.235 | -4.87447 | $-5.46071 \times 10^{-4}$ | $4.86312 \times 10^{-4}$ |
| -0.323 | -5.05405 | -0.00614 | $8.53415 \times 10^{-4}$ |

TABLE S2: Parameters obtained from fitting a cubic polynomial $y = Bx + Cx^2 + Dx^3$ for the wire setup as shown in Figure 10(b).

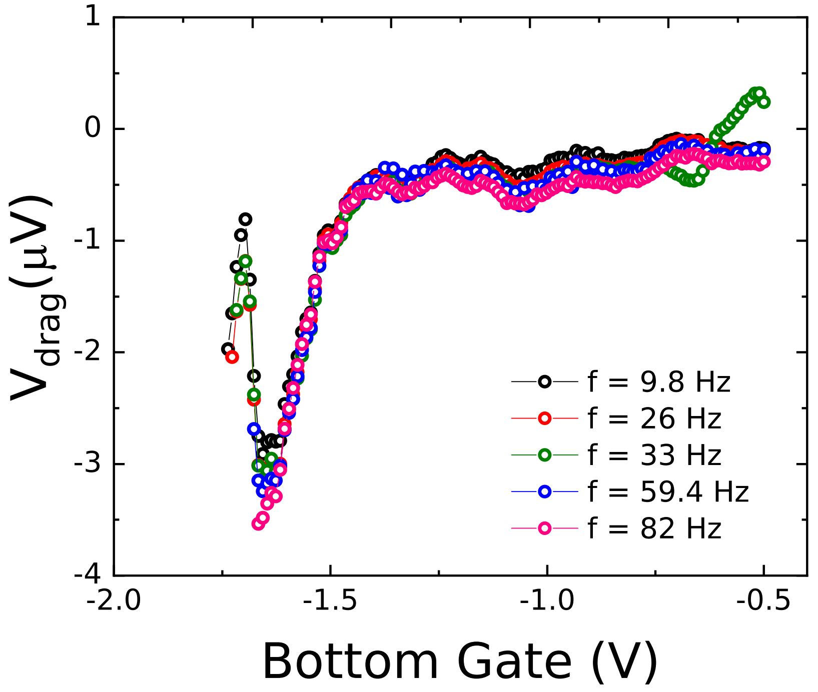


FIG. S4: Drag resistance as a function of right gate voltage for different frequencies, with left gate at -0.85 V and middle gate at 0.15 V.

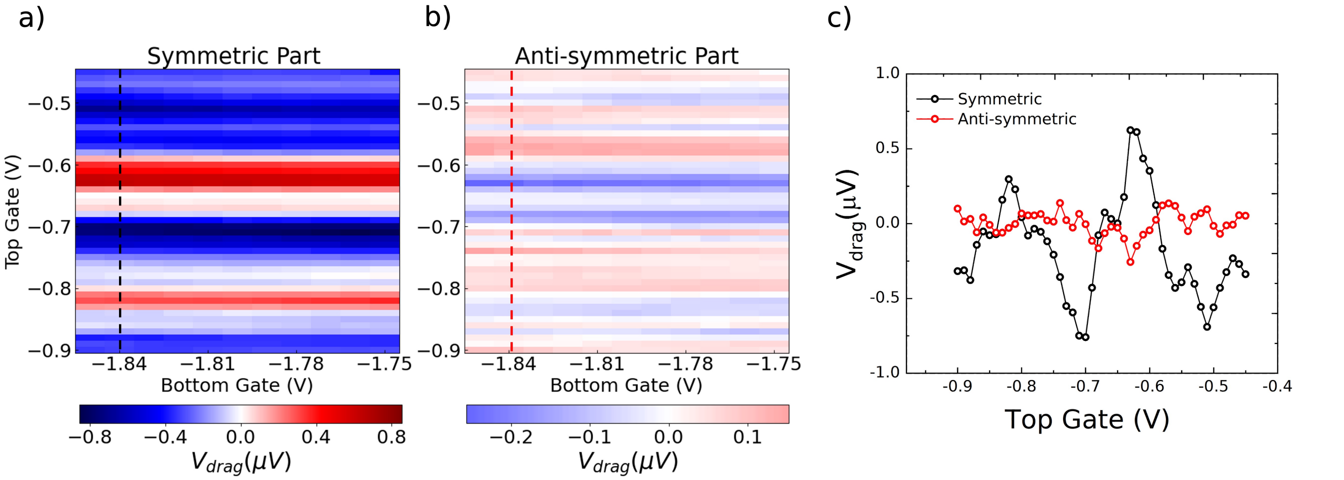


FIG. S5: a) Symmetric and b) Anti-symmetric drag components taken from Fig. 3(c) and (d) of the main text. c) The line trace of symmetric and anti-symmetric drag component at $V_B$= -1.84 V

## VI. AC CURRENT DEPENDENCE

Tables S3 and S4 report the fitting parameters for all the dependencies presented in Fig. 6(a) and (b) of the main text, respectively.

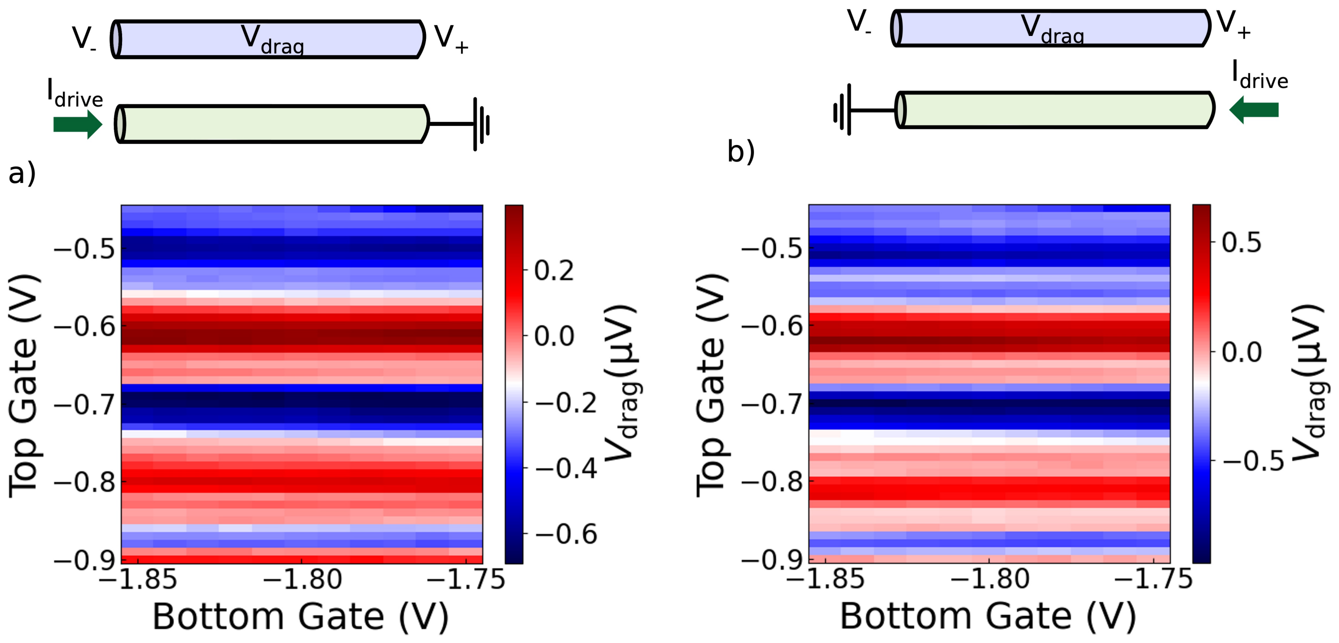


FIG. S6: AC Drag as a function of top and bottom gate voltages at 200 mK with a) top wire as drag wire and bottom wire as drive wire. b) Same as a) with direction of current reversed.

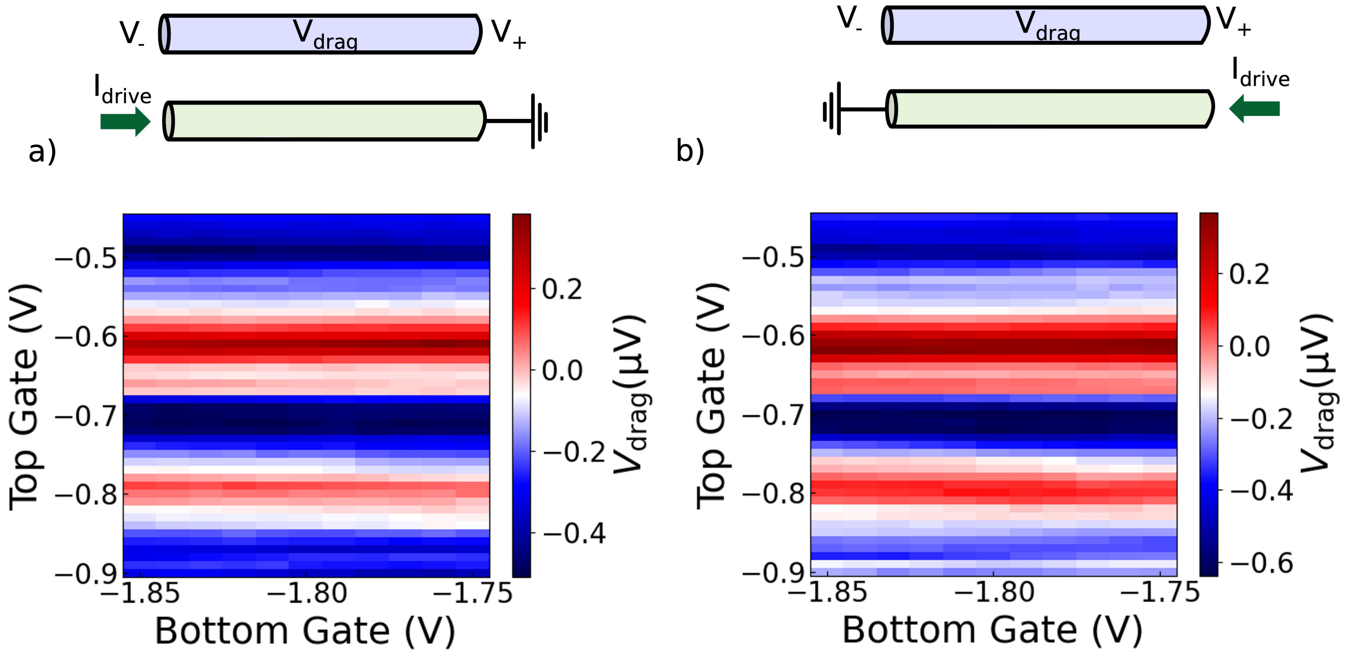


FIG. S7: AC Drag as a function of top and bottom gate voltages at 500 mK with a) top wire as drag wire and bottom wire as drive wire. b) Same as a) with direction of current reversed.

## VII. MAGNETIC DEPOPULATION

We estimate the 1D electron density of our lateral device from magnetic depopulation measurements. The two-dimensional electron gas (2DEG) is subjected to a perpendicular magnetic field at low temperature, which results in oscillations (Shubnikov-de Haas oscillations) due to the quantization of electron orbits in the presence of a magnetic field. The sublevel indices, which are the local minimas in the Shubnikov-de Haas oscillations, are then plotted against

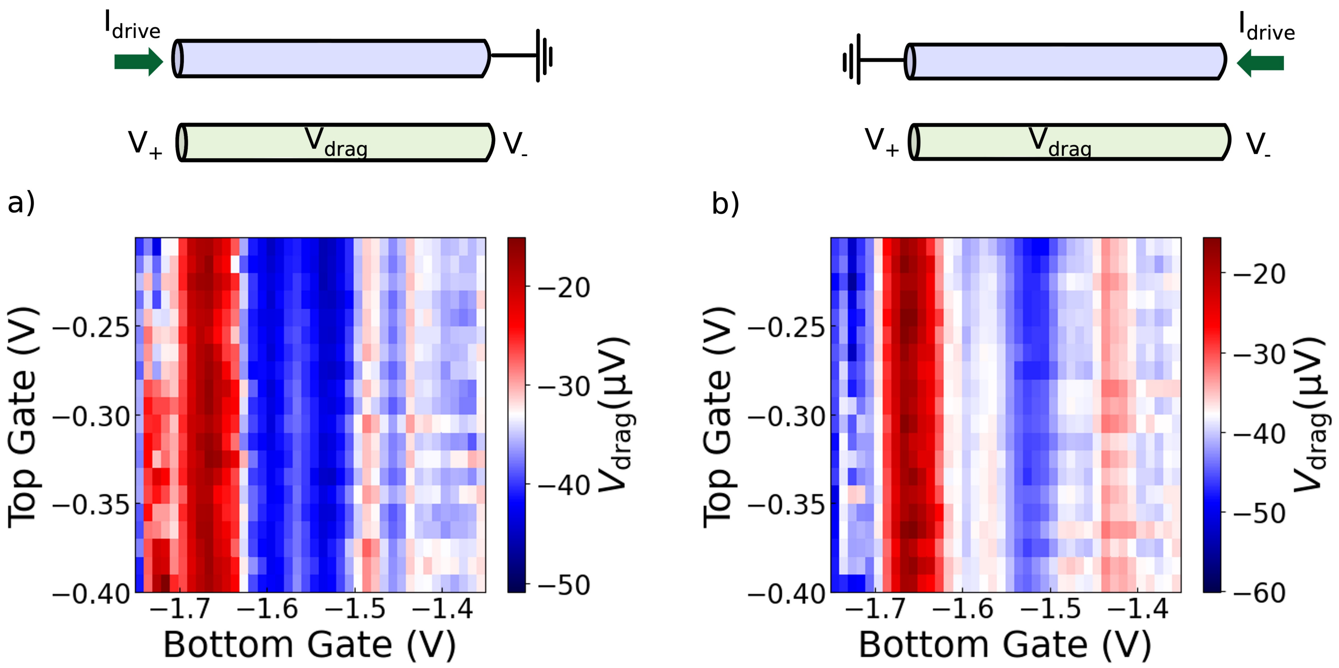


FIG. S8: DC Drag as a function of top and bottom gate voltages at 200 mK with a) top wire as drag wire and bottom wire as drive wire. b) Same as a) with direction of current reversed.

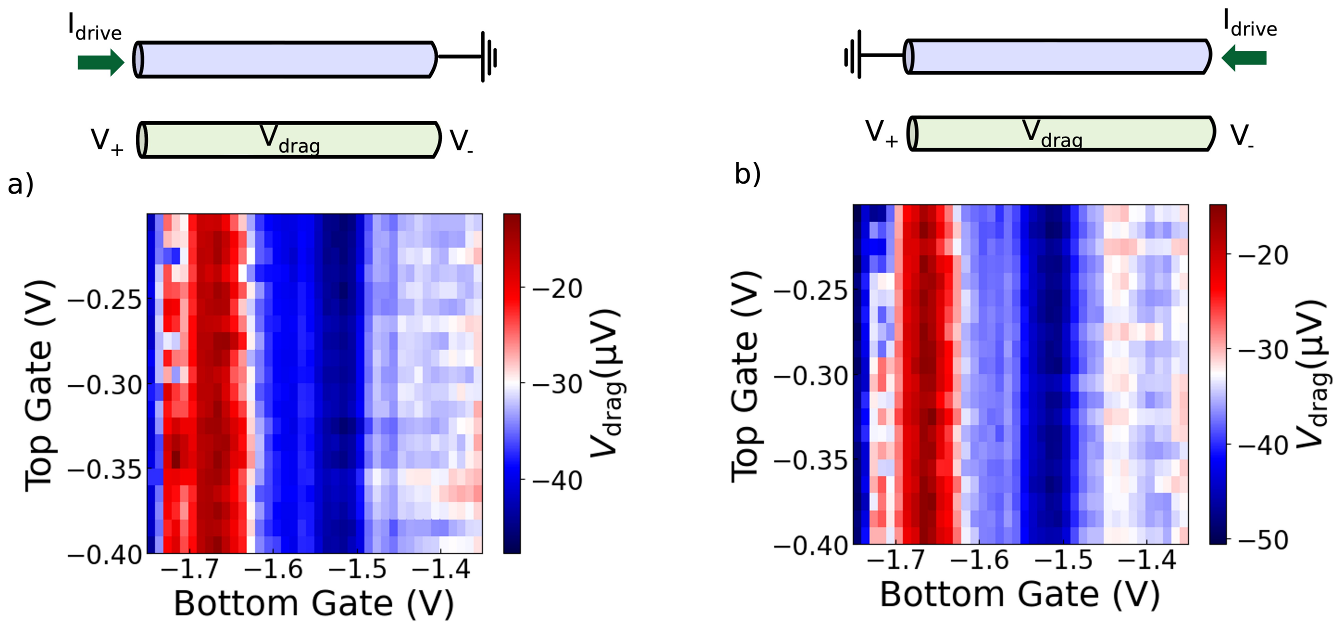


FIG. S9: DC Drag as a function of top and bottom gate voltages at 500 mK with a) top wire as drag wire and bottom wire as drive wire. b) Same as a) with direction of current reversed.

the inverse of the magnetic field, and we used the following equations [1] to extract the 1D electron density.

$$n \approx [\frac{3\pi}{4} N_e^{1D} (\frac{\hbar}{2m^*})^{\frac{1}{2}}]^{2/3} \frac{1}{\omega_c} \tag{1}$$

$$N_e^{1D} \approx \frac{2}{\pi} \sqrt{\frac{2m^*}{\hbar}} \frac{\omega^{3/2}}{\omega_0} \frac{2}{3} n^{2/3} \tag{2}$$

where, n in the subband index, $m^* = 0.067 m_e$ is the effective mass in GaAs, $m_e$ is the free electron mass $N_e^{1D}$ is

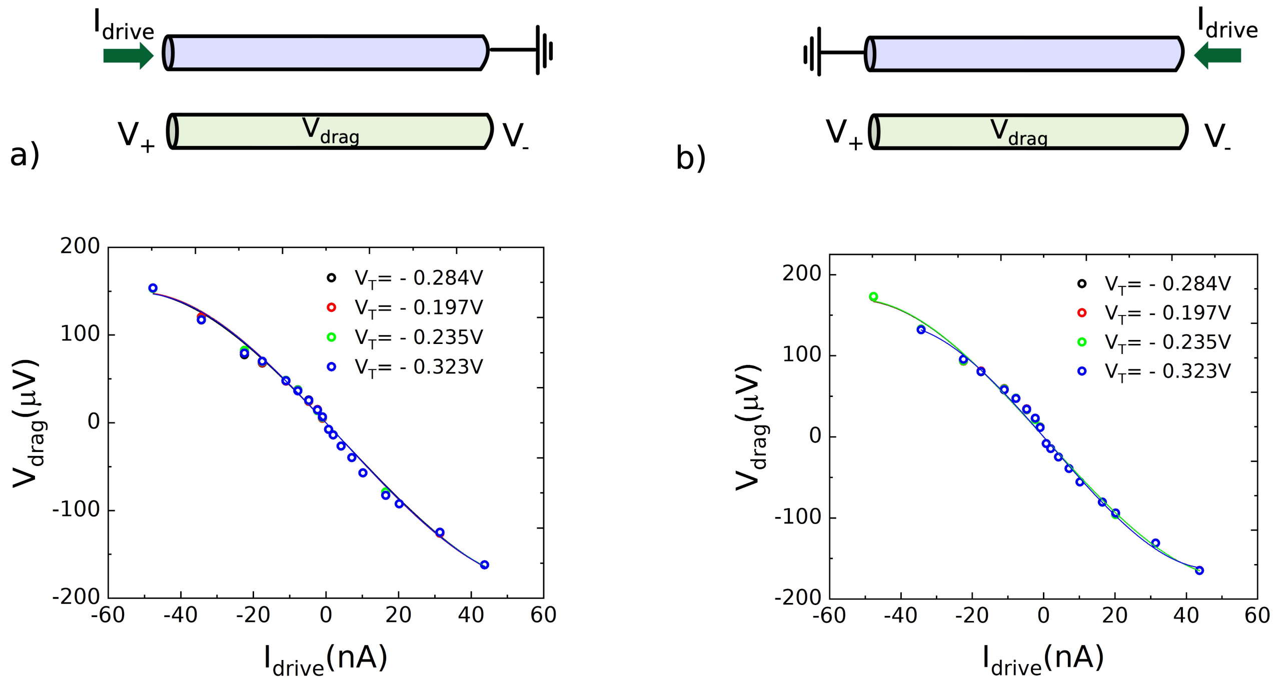


FIG. S10: DC Drag as a function of drive current with different top gate voltages ($V_T$). a) The top wire is the drive wire and the bottom wire is the drag wire. b) Same as a) with the direction of the current reversed.

| $V_T(V)$ | B ($\mu V/nA$) | C ($\mu V/nA^2$) | D ($\mu V/nA^3$) |
|---|---|---|---|
| -1.32 | 0.0296419 | $-4.14207 \times 10^{-3}$ | $7.75002 \times 10^{-5}$ |
| -1.37 | $-0.0889766$ | $-1.649229 \times 10^{-2}$ | $2.17837 \times 10^{-4}$ |
| -1.45 | $-0.192284$ | $1.79043 \times 10^{-2}$ | $-2.19399 \times 10^{-4}$ |
| -1.58 | 0.145748 | $-2.38961 \times 10^{-2}$ | $2.88497 \times 10^{-4}$ |
| -1.52 | 0.145184 | $1.44364 \times 10^{-2}$ | $-2.29188 \times 10^{-4}$ |

TABLE S3: Parameters obtained from fitting a cubic polynomial $y = Bx + Cx^2 + Dx^3$ for the wire setup as shown in Figure 6(a) of the main text.

| $V_T(V)$ | B ($\mu V/nA$) | C ($\mu V/nA^2$) | D ($\mu V/nA^3$) |
|---|---|---|---|
| -1.32 | $-0.259559$ | -1.36639 $\times 10^{-2}$ | $-1.61297 \times 10^{-4}$ |
| -1.37 | $-0.329161$ | -7.91749 $\times 10^{-3}$ | $-9.38976 \times 10^{-5}$ |
| -1.45 | 0.158522 | $3.97888 \times 10^{-3}$ | $-5.28681 \times 10^{-5}$ |
| -1.58 | $-1.85417$ | -3.27673 $\times 10^{-2}$ | $-2.22791 \times 10^{-4}$ |
| -1.52 | 0.46061 | $9.60223 \times 10^{-3}$ | $-1.23449 \times 10^{-4}$ |

TABLE S4: Parameters obtained from fitting a cubic polynomial $y = Bx + Cx^2 + Dx^3$ for the wire setup as shown in Figure 6(b) of the main text.

the 1D electron density, $\omega_c$ is the cyclotron frequency $= |e|B/m^*$ and $\omega = \sqrt{\omega_c^2 + \omega_0^2}$.

Fig. S11 shows the Shubnikov-de Haas oscillations and the n vs 1/B plot when 5 subbands are populated in the wires. Similar calculations were done at 6 subbands population in the wire.

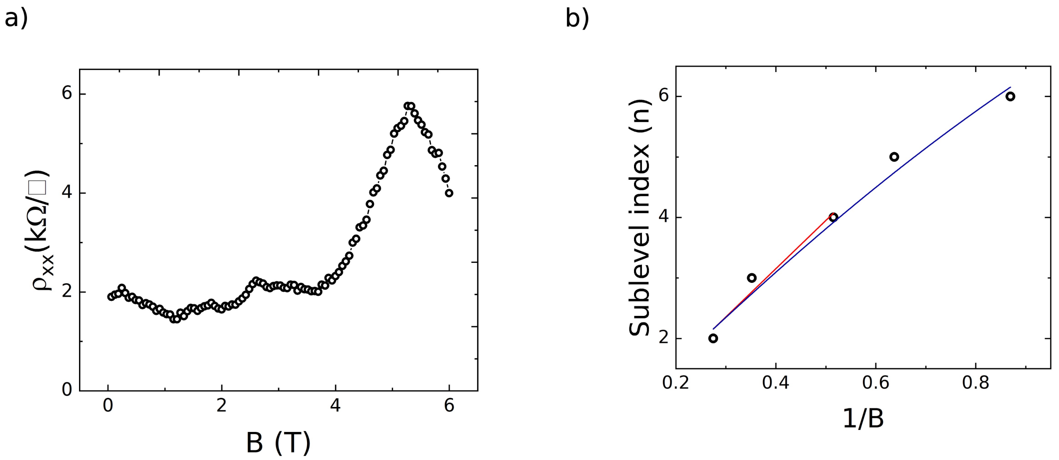


FIG. S11: a) Experimental data showing Shubnikov-de Haas oscillations in the lateral device. b) Sublevel index n vs inverse magnetic field, with linear fit (Eq. 1) in the high magnetic field regime (red line), which yields $\omega_0 = 1.54 \times 10^{12}$ and a non-linear fit (Eq. 2) (blue line) resulting in the 1D density of $N_e^{1D} = 8.94 \times 10^8 m^{-1}$ .

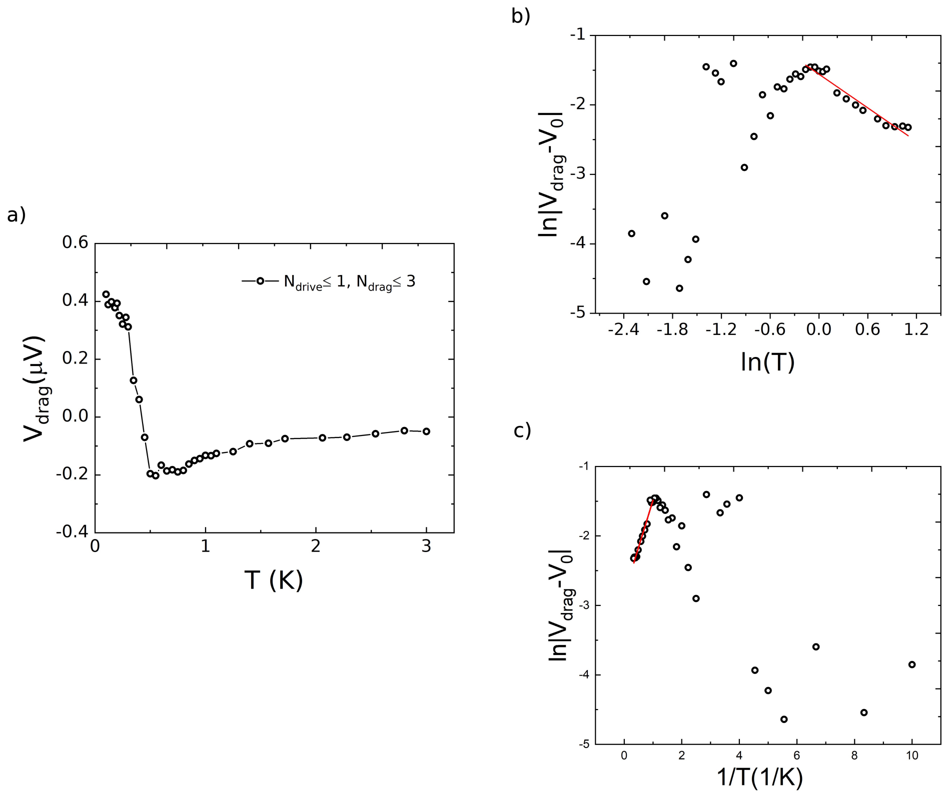


FIG. S12: a) Temperature dependence of the drag signal with $N_{drive} \leq 1$ and $N_{drag} \leq 3$. b) Log-log plot of drag voltage and temperature and the offset $V_0 = -0.00713\,\mu V$ and c) Arrhenius plot of drag voltage and temperature and the offset $V_0 = -0.00713\,\mu V$ for the temperature dependence shown in (a).

## VIII. TEMPERATURE DEPENDENCE

In addition to the fittings shown in Fig. 7 b) and c) of the main text, we performed a similar analysis for the temperature data acquired when $N_{drive} \leq 1$ and $N_{drag} \leq 3$ (red curve in Fig. 7 (a) of main text). Fig. S12 shows the

drag signal as a function of temperature, along with the log-log plot and the Arrhenius plot. The exponents for the fittings were calculated as $V_{drag} \propto T^{\alpha}$; $\alpha = -0.8 \pm 0.2$ for the power law function and $V_{drag} \propto e^{\frac{\beta}{T}}$; $\beta = -1.35 \pm 0.2$. The value of the offset $V_0$ was estimated from a standard fit in the high temperature regime.

## IX. CALCULATION OF THE ERROR BARS OF THE FITTING PARAMETERS

The error bars of the fitting parameters were determined using a bootstrap Monte-Carlo method. The standard deviation of the noise in our data was utilized as the error on individiual points if fig. 7(a). Assuming a normal distribution with the reported value as the mean and the error as the standard deviation, we randomly generated a new series of points. We generated 10000 such datasets and then fitted the power law $V_D = AT^{\alpha} + V_0$ to each of these datasets. The standard deviation of the calculated exponents $\alpha$ of all the dataset was then used as the error on the exponent. A similarly process was used to find error bars on the Arrhenius plot. For the temperature dependence with $N_{drive} \leq 1$ and $N_{drag} \leq 4$ (black curve in Fig. 7 (a) of main text), the fitting region was $T \geq 0.45K$ and with $N_{drive} \leq 1$ and $N_{drag} \leq 3$ (red curve in Fig. 7 (a) of main text), the fitting region was $T \geq 0.8K$.

[1] Berggren, K.-F, Ross, G., and van Houten, H., Characterization of very narrow quasi-one-dimensional quantum channels, Phys. Rev. B **37**, 10118 (1988).
